# Supplementary material for: Learning Deblurring Texture Prior from Unpaired Data with Diffusion Model
Source: arXiv:2507.13599 source file (2025-07-18)

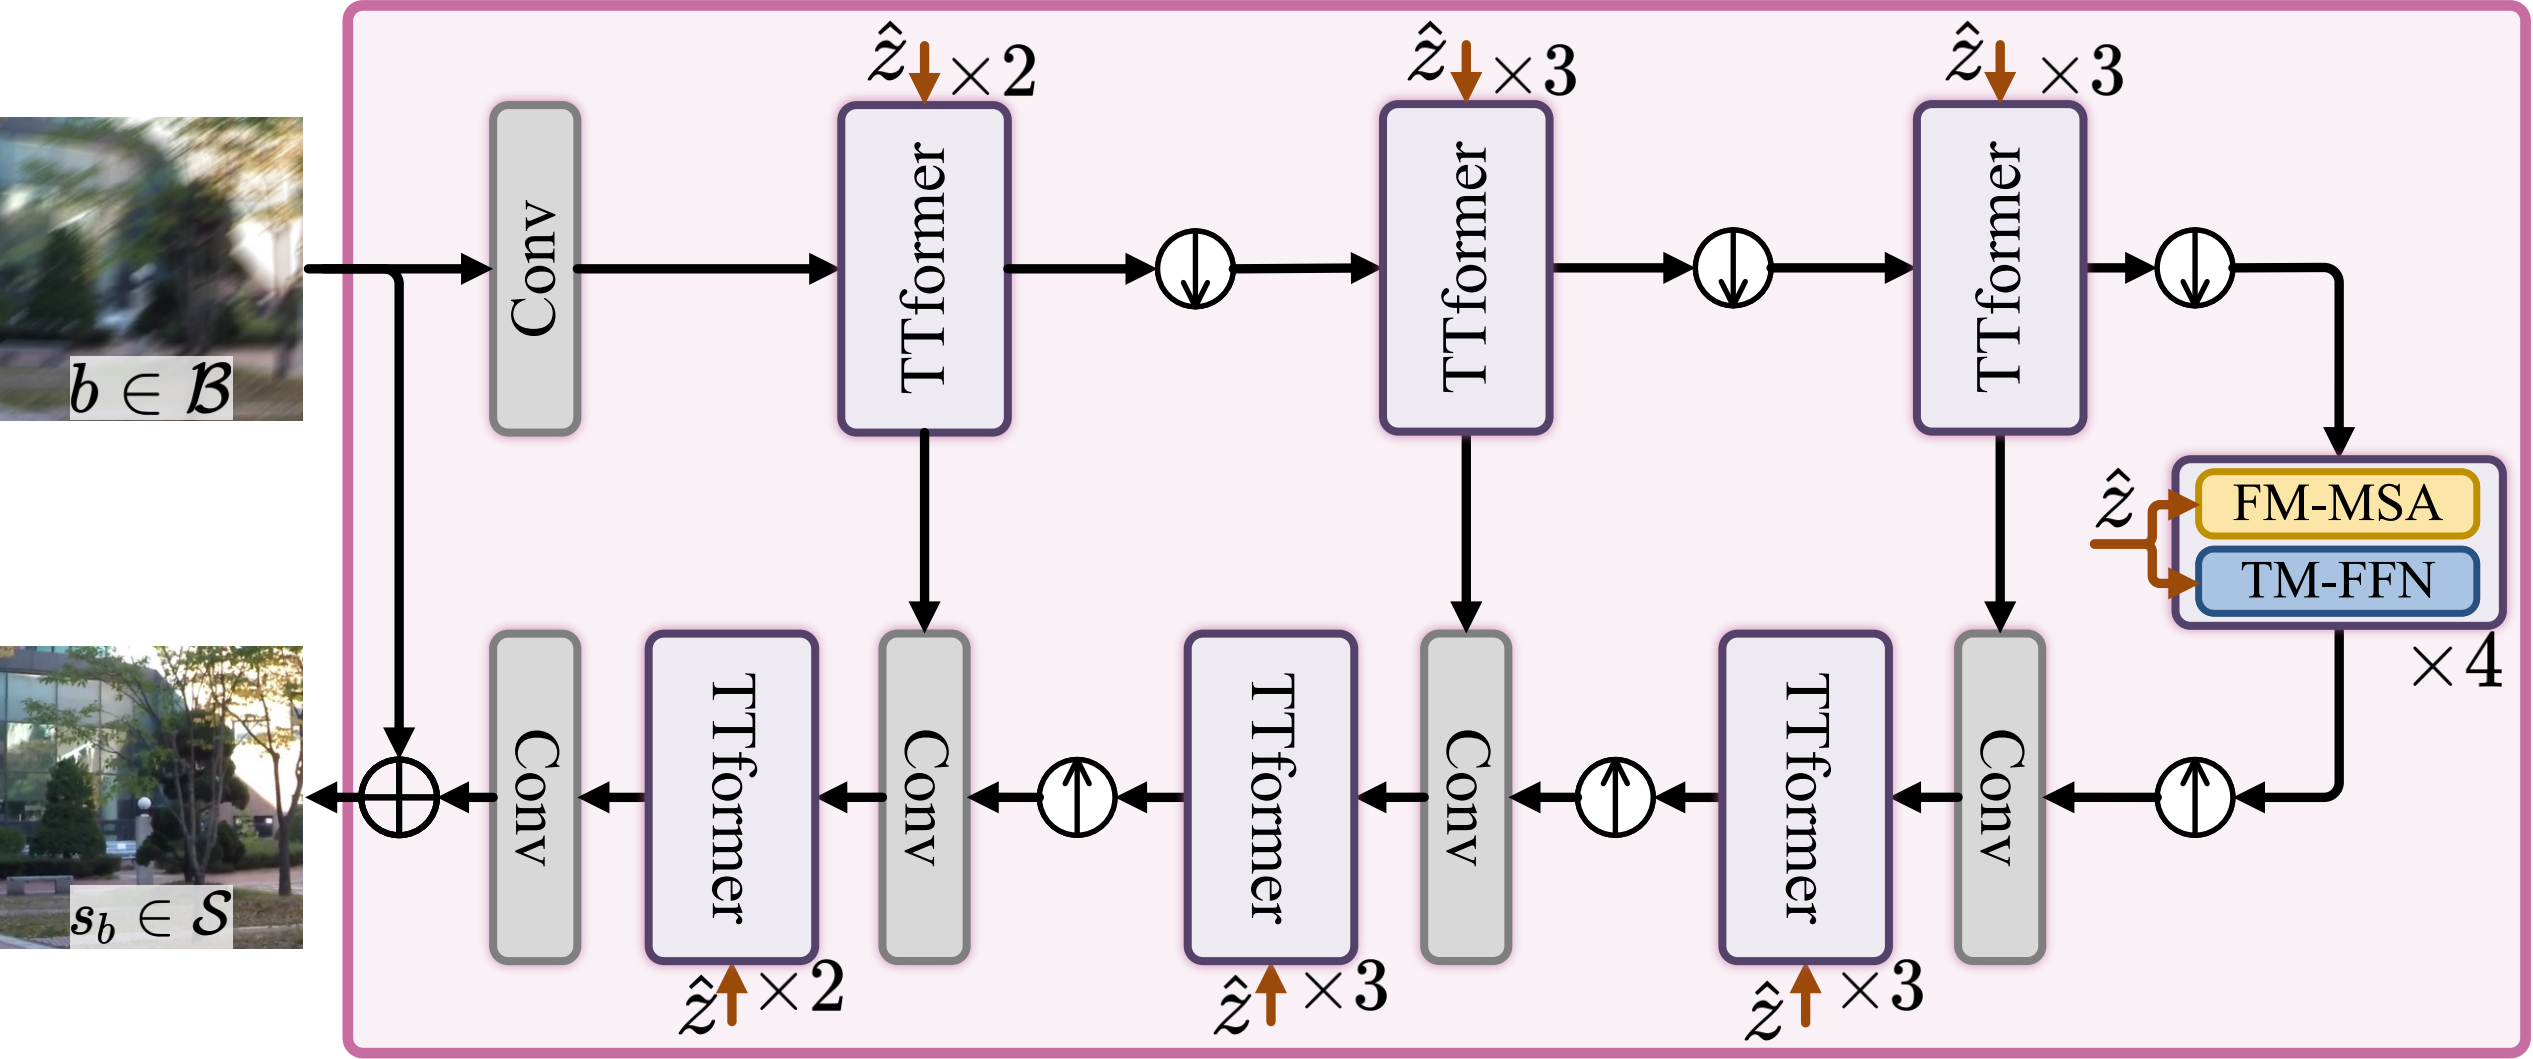



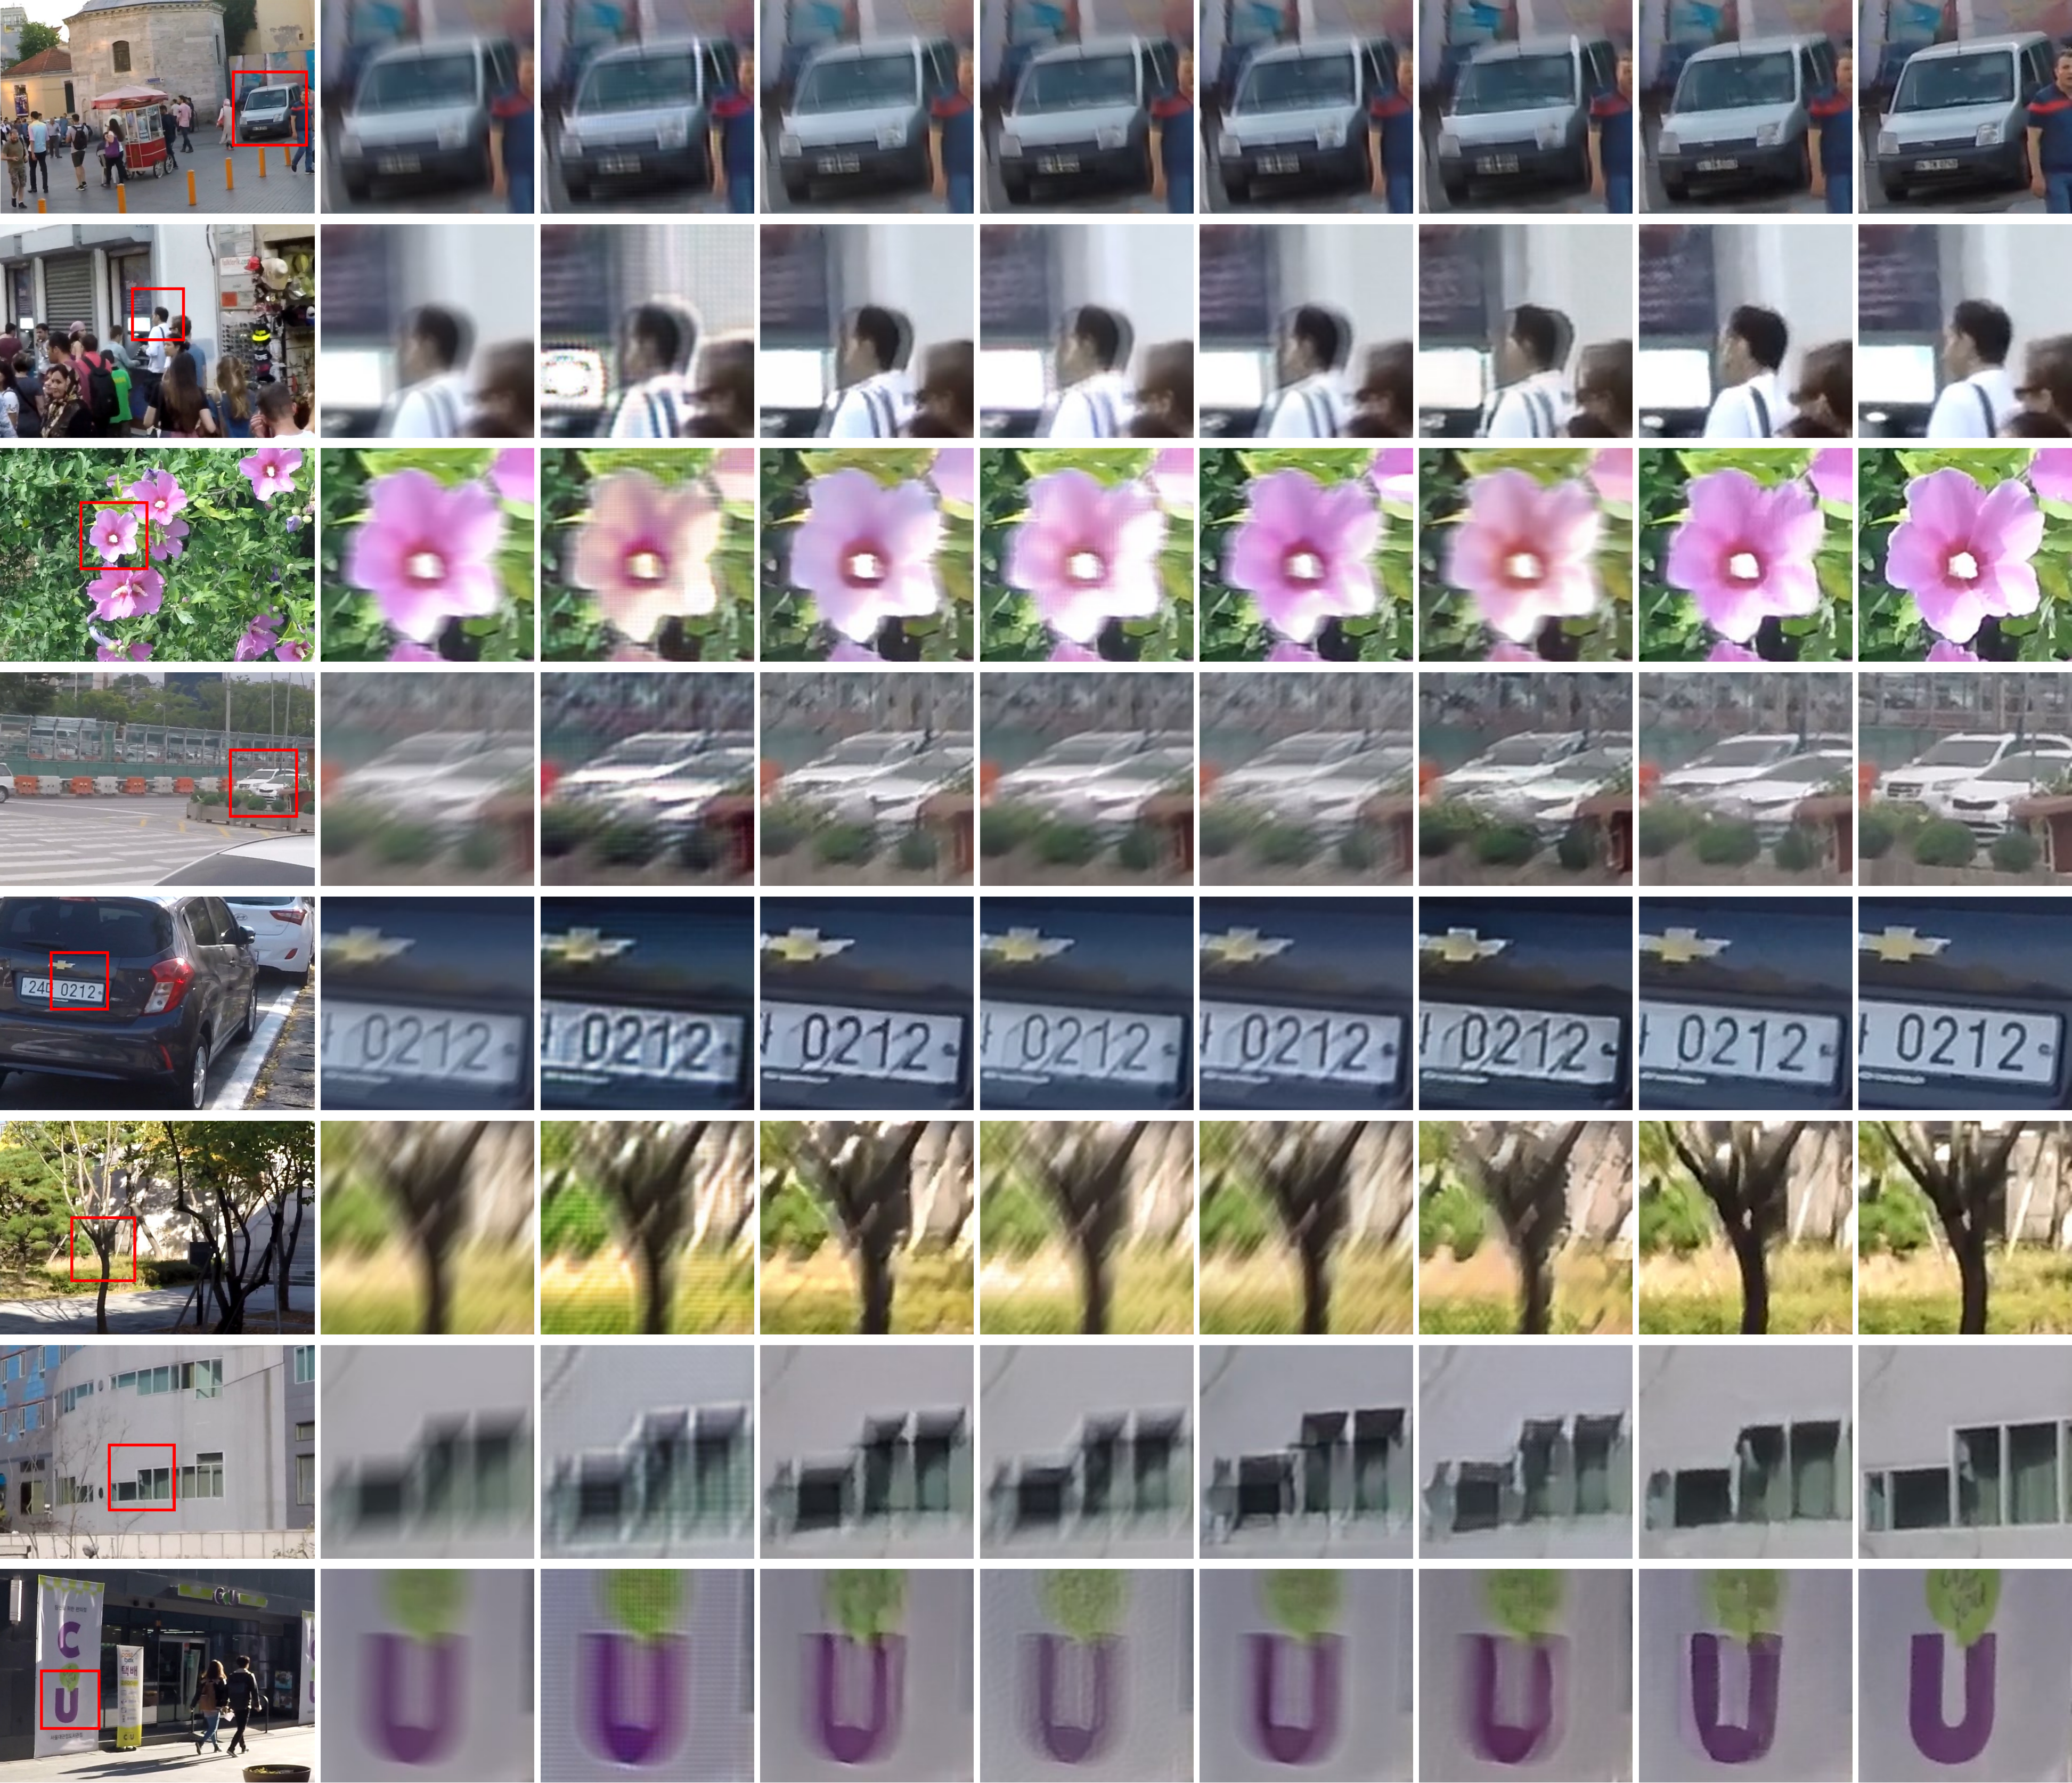

Blurry

CycleGAN

UID-GAN

LIR

FCL-GAN

UCL

Ours

GT



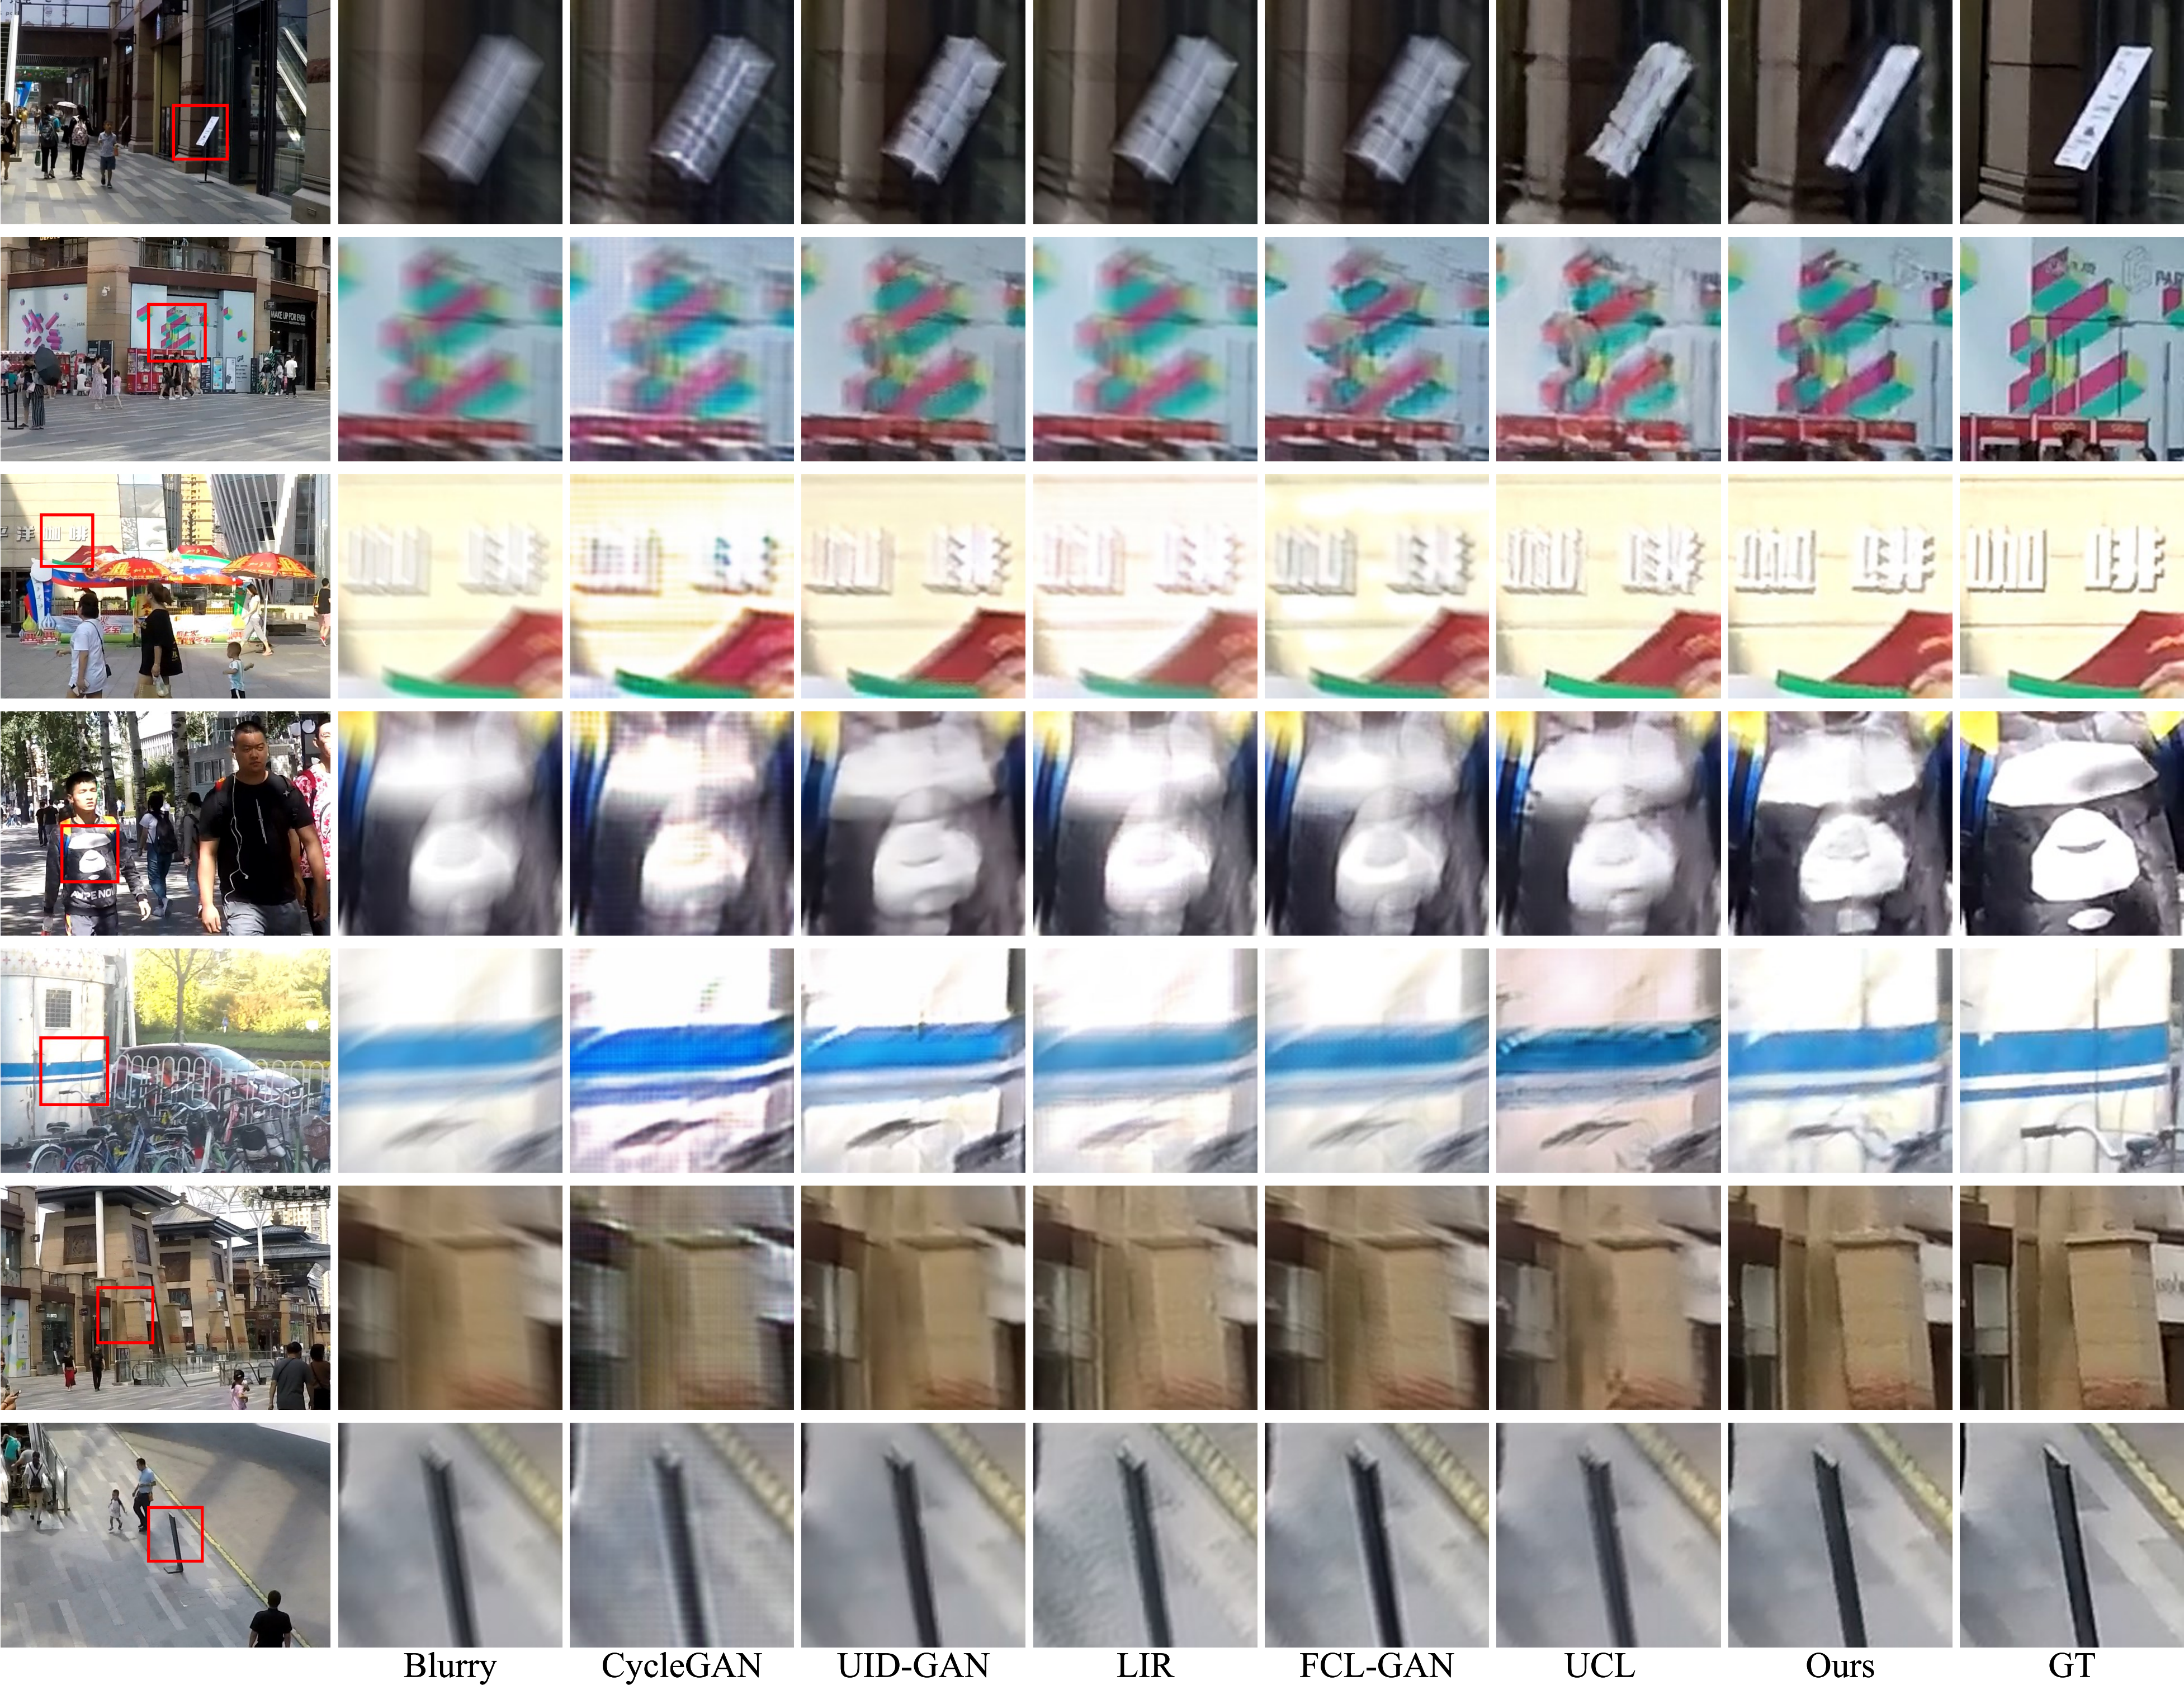



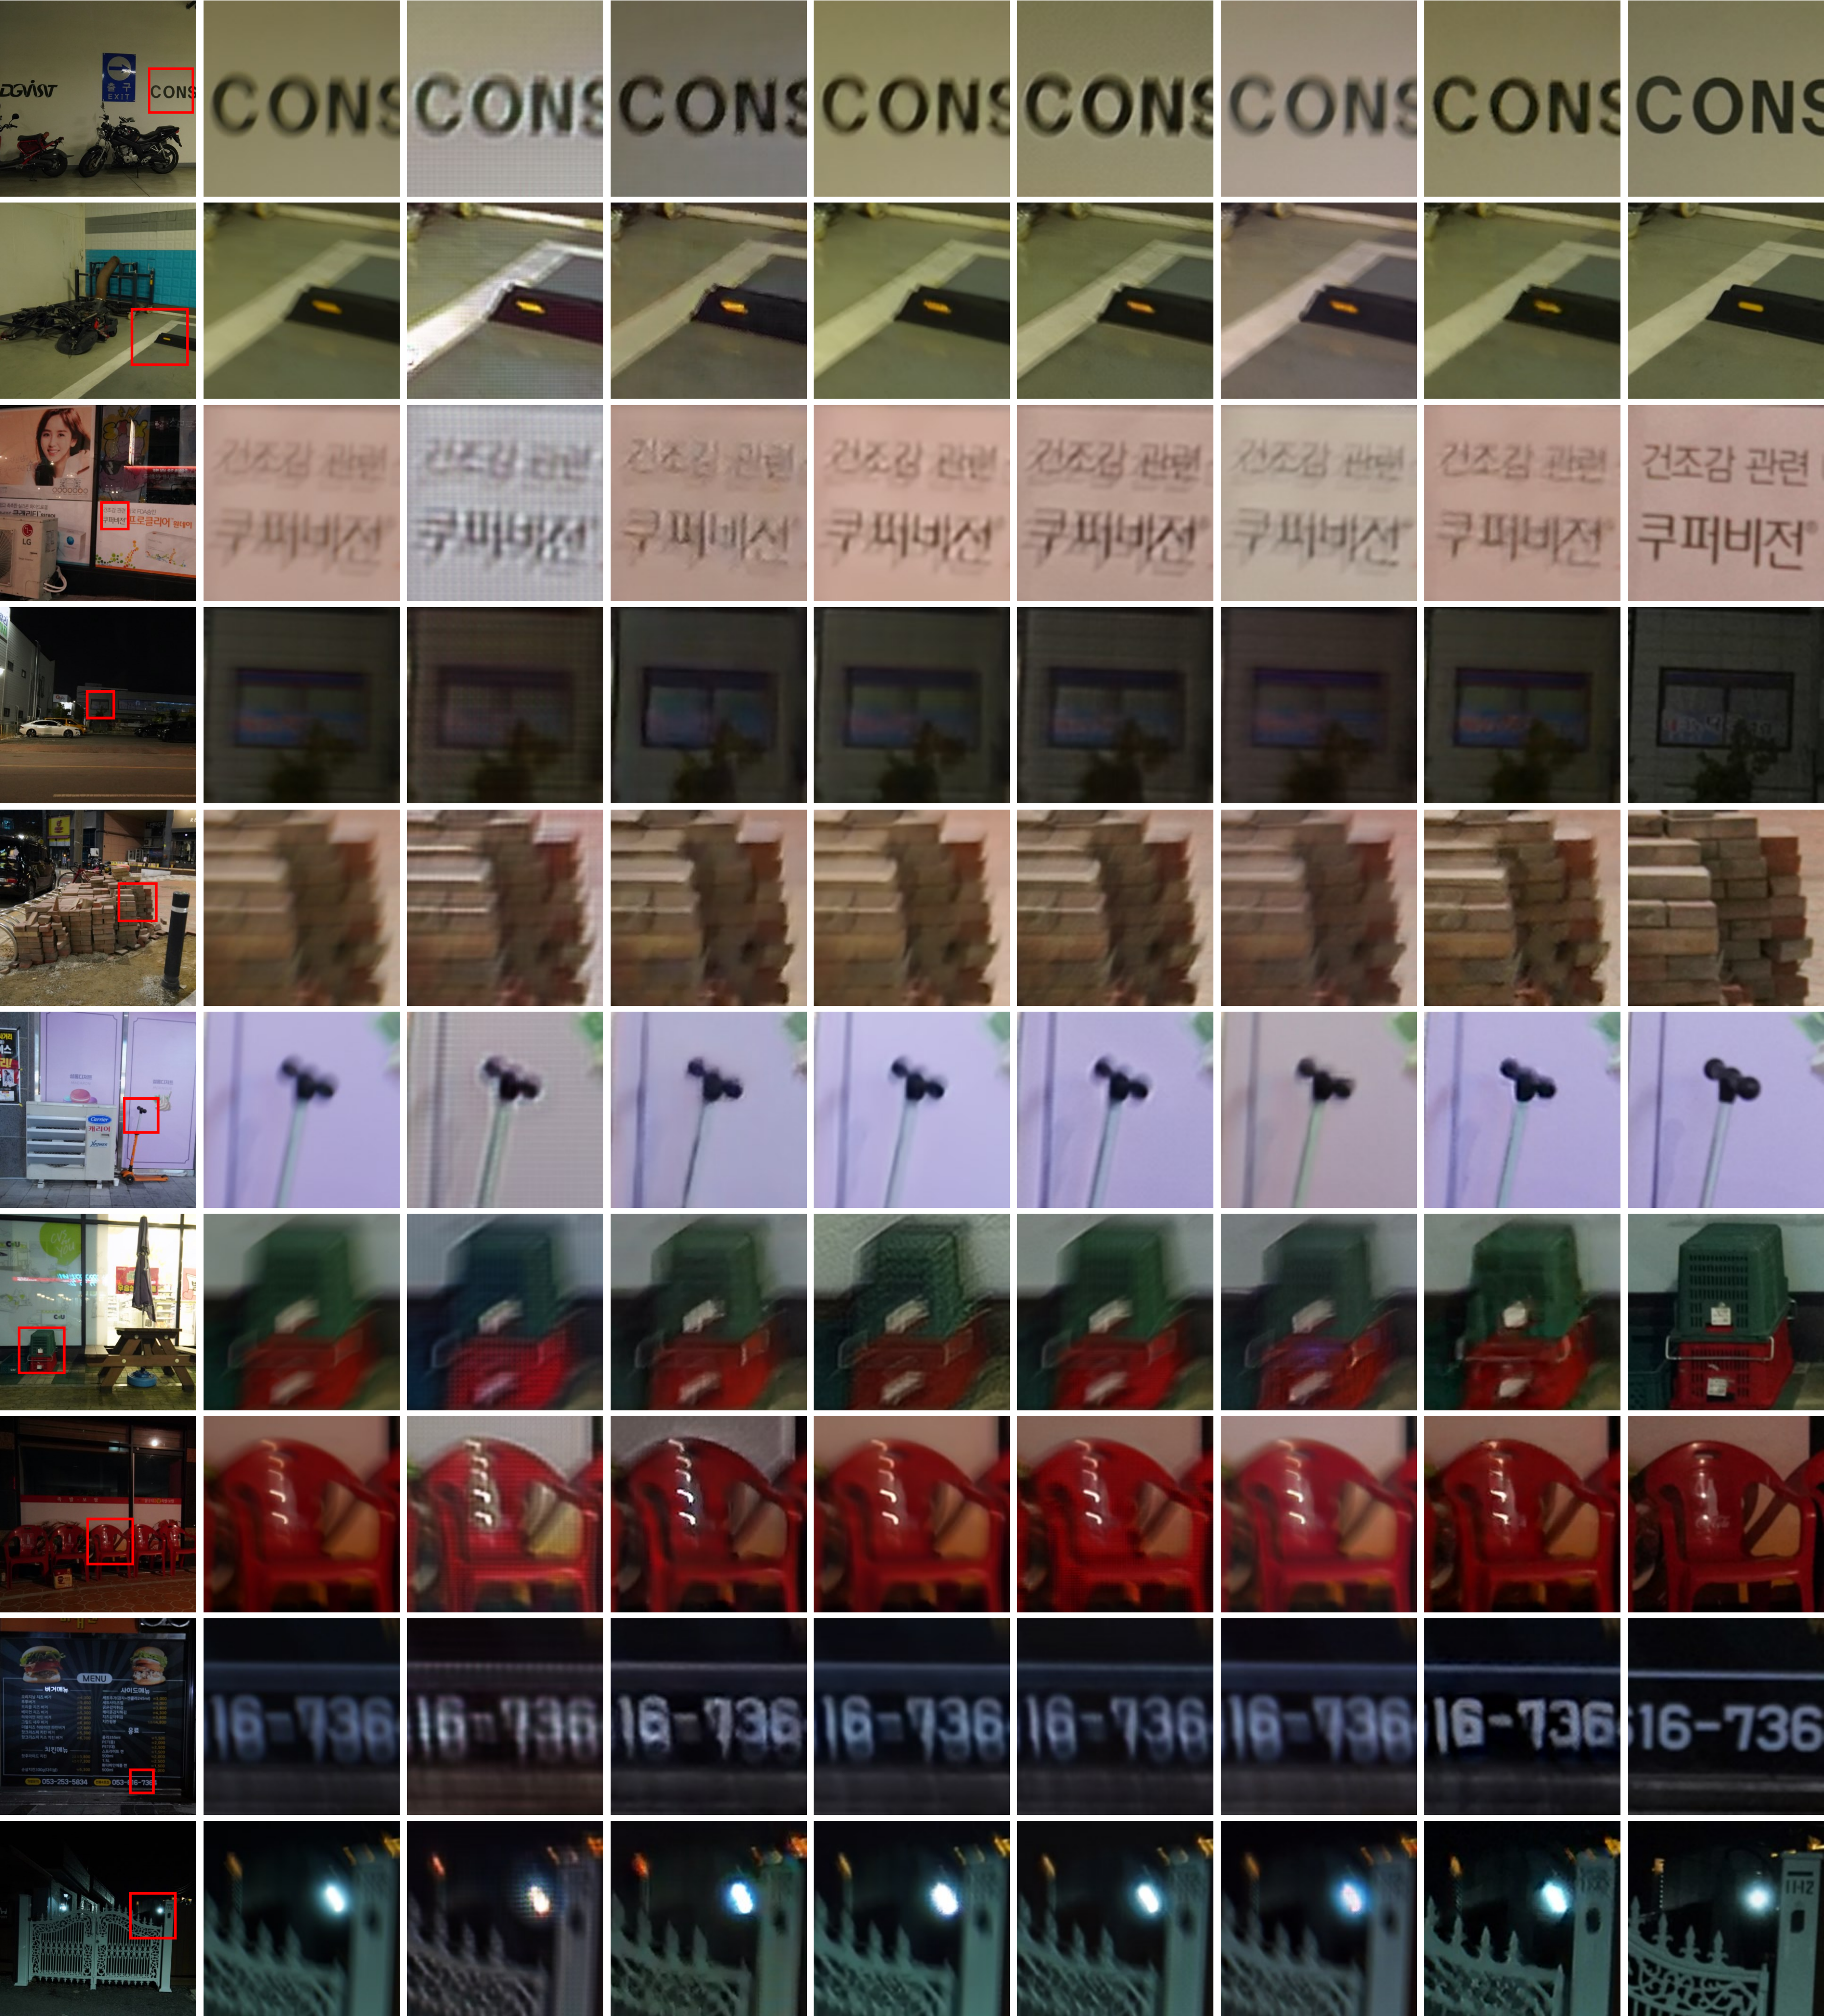

Blurry

CycleGAN

UID-GAN

LIR

FCL-GAN

UCL

Ours

GT



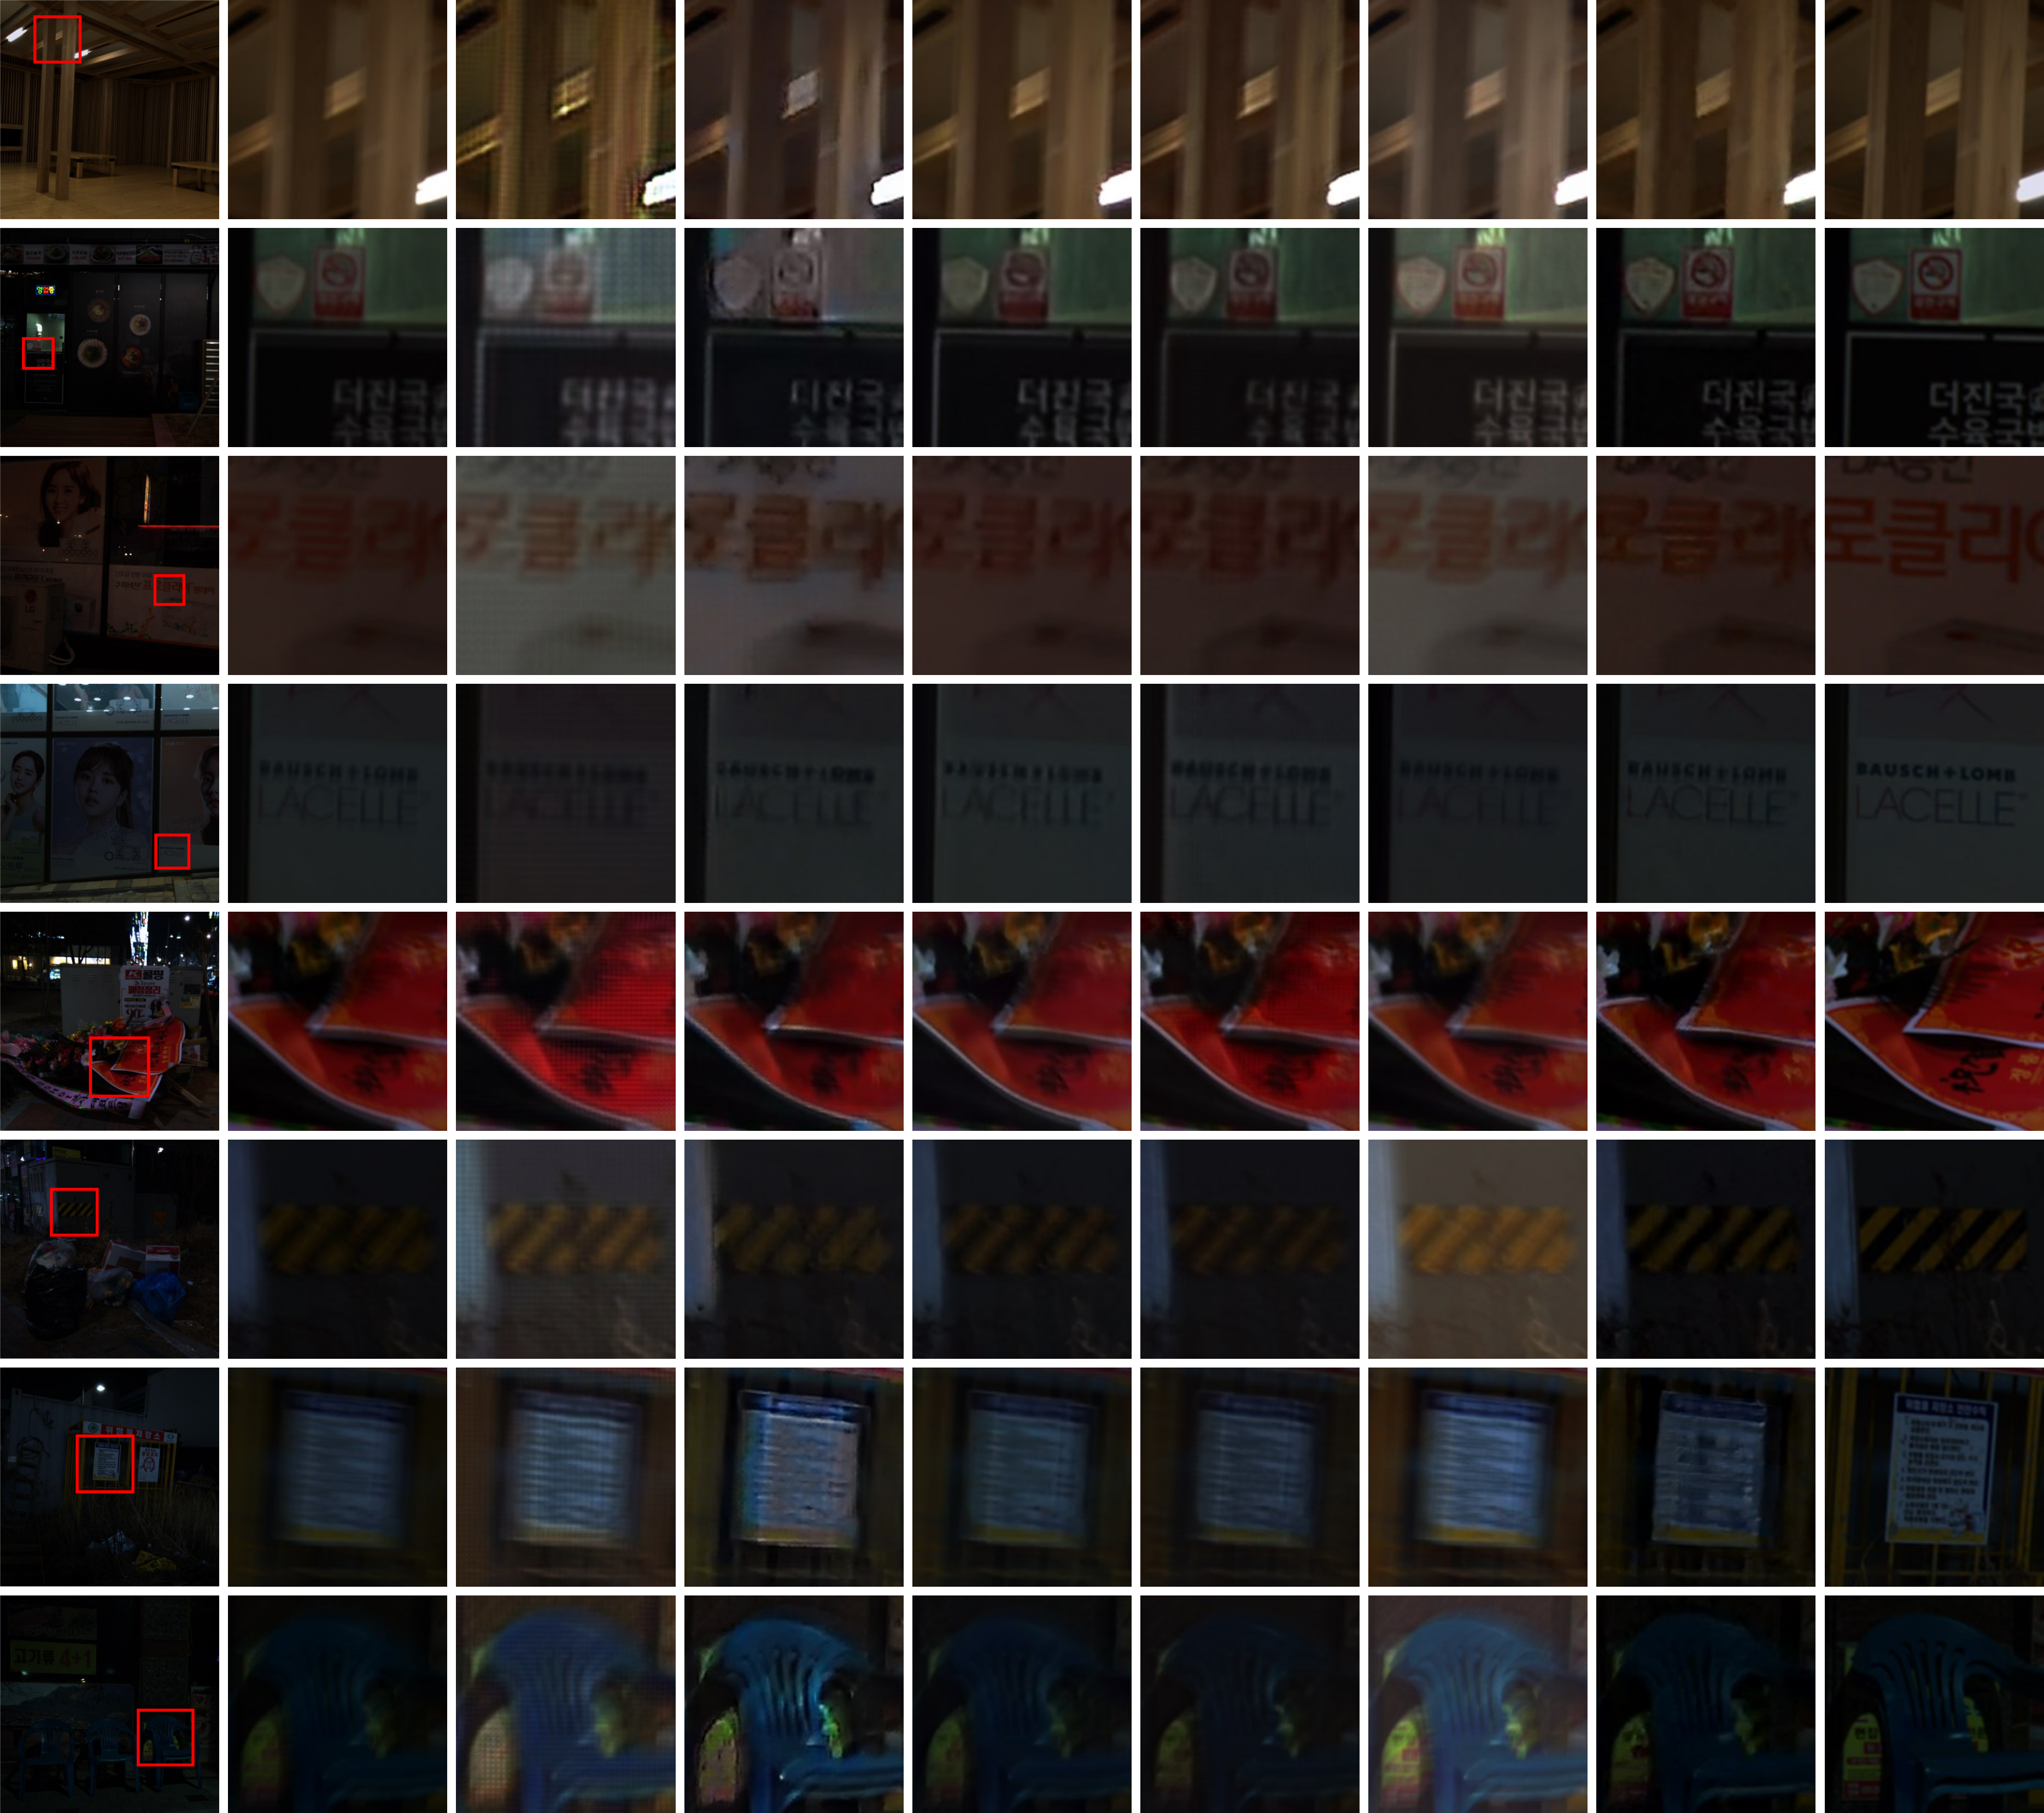



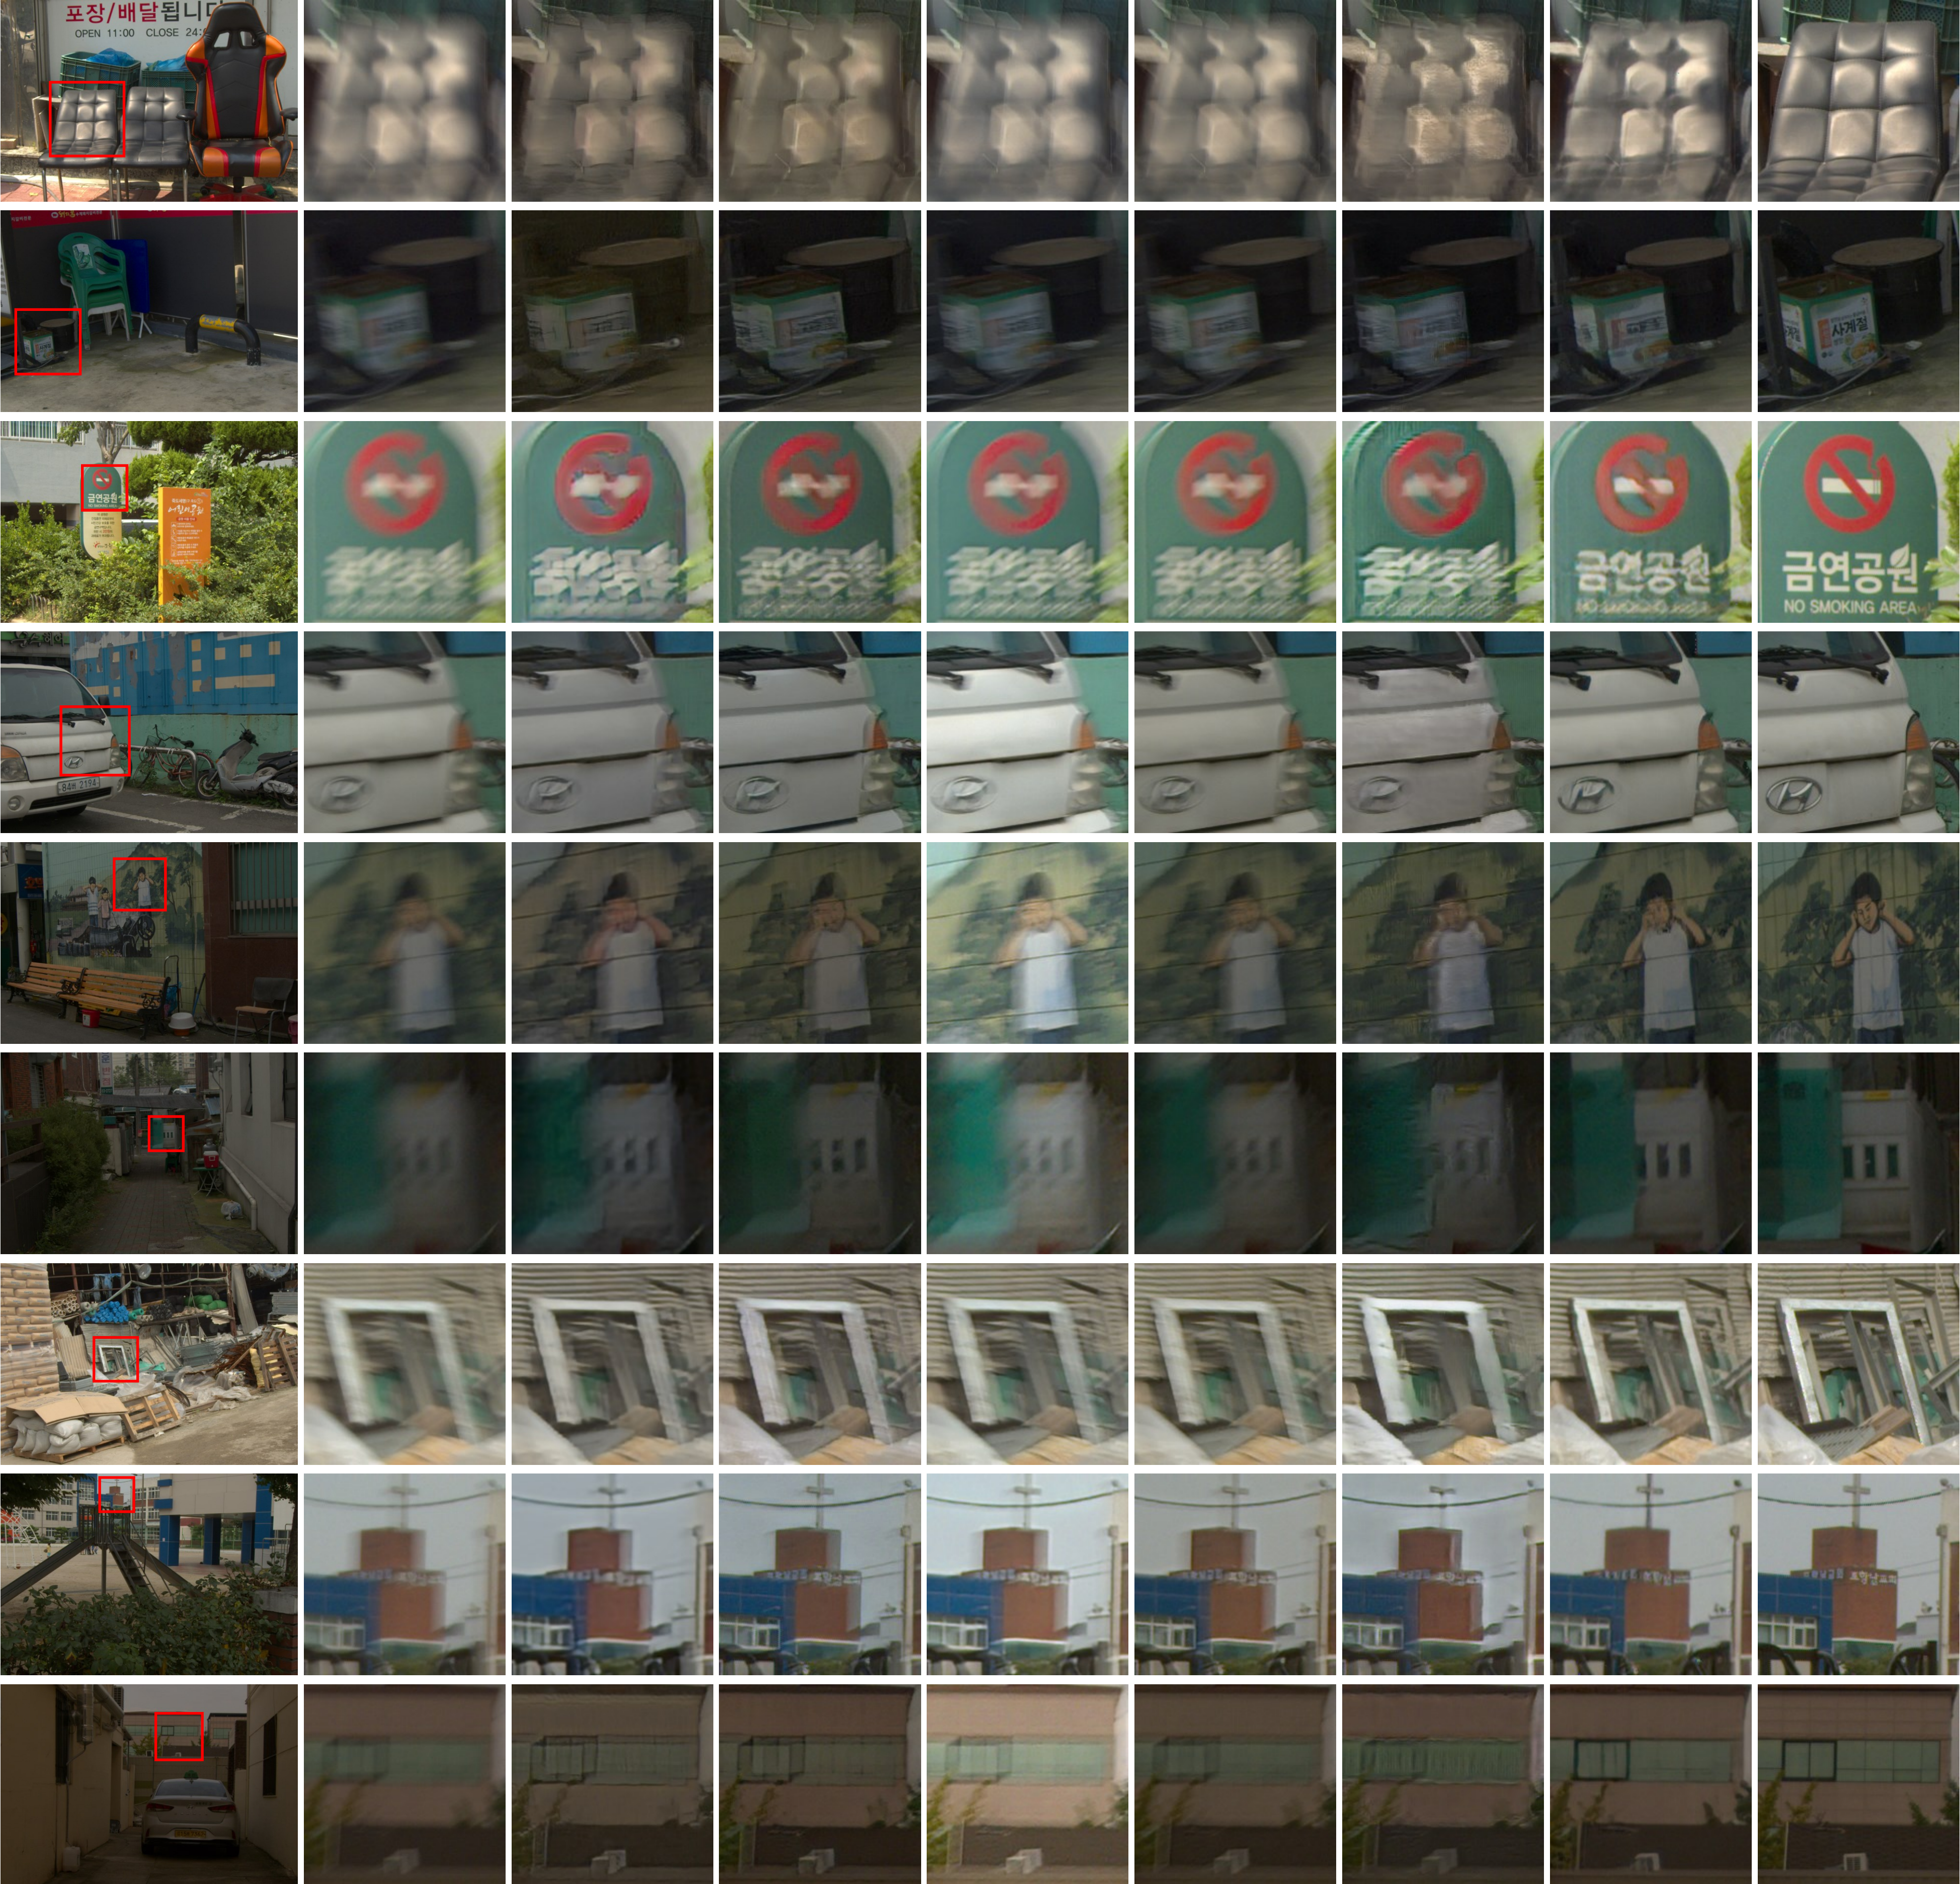

Blurry

CycleGAN

UID-GAN

LIR

FCL-GAN

UCL

Ours

GT



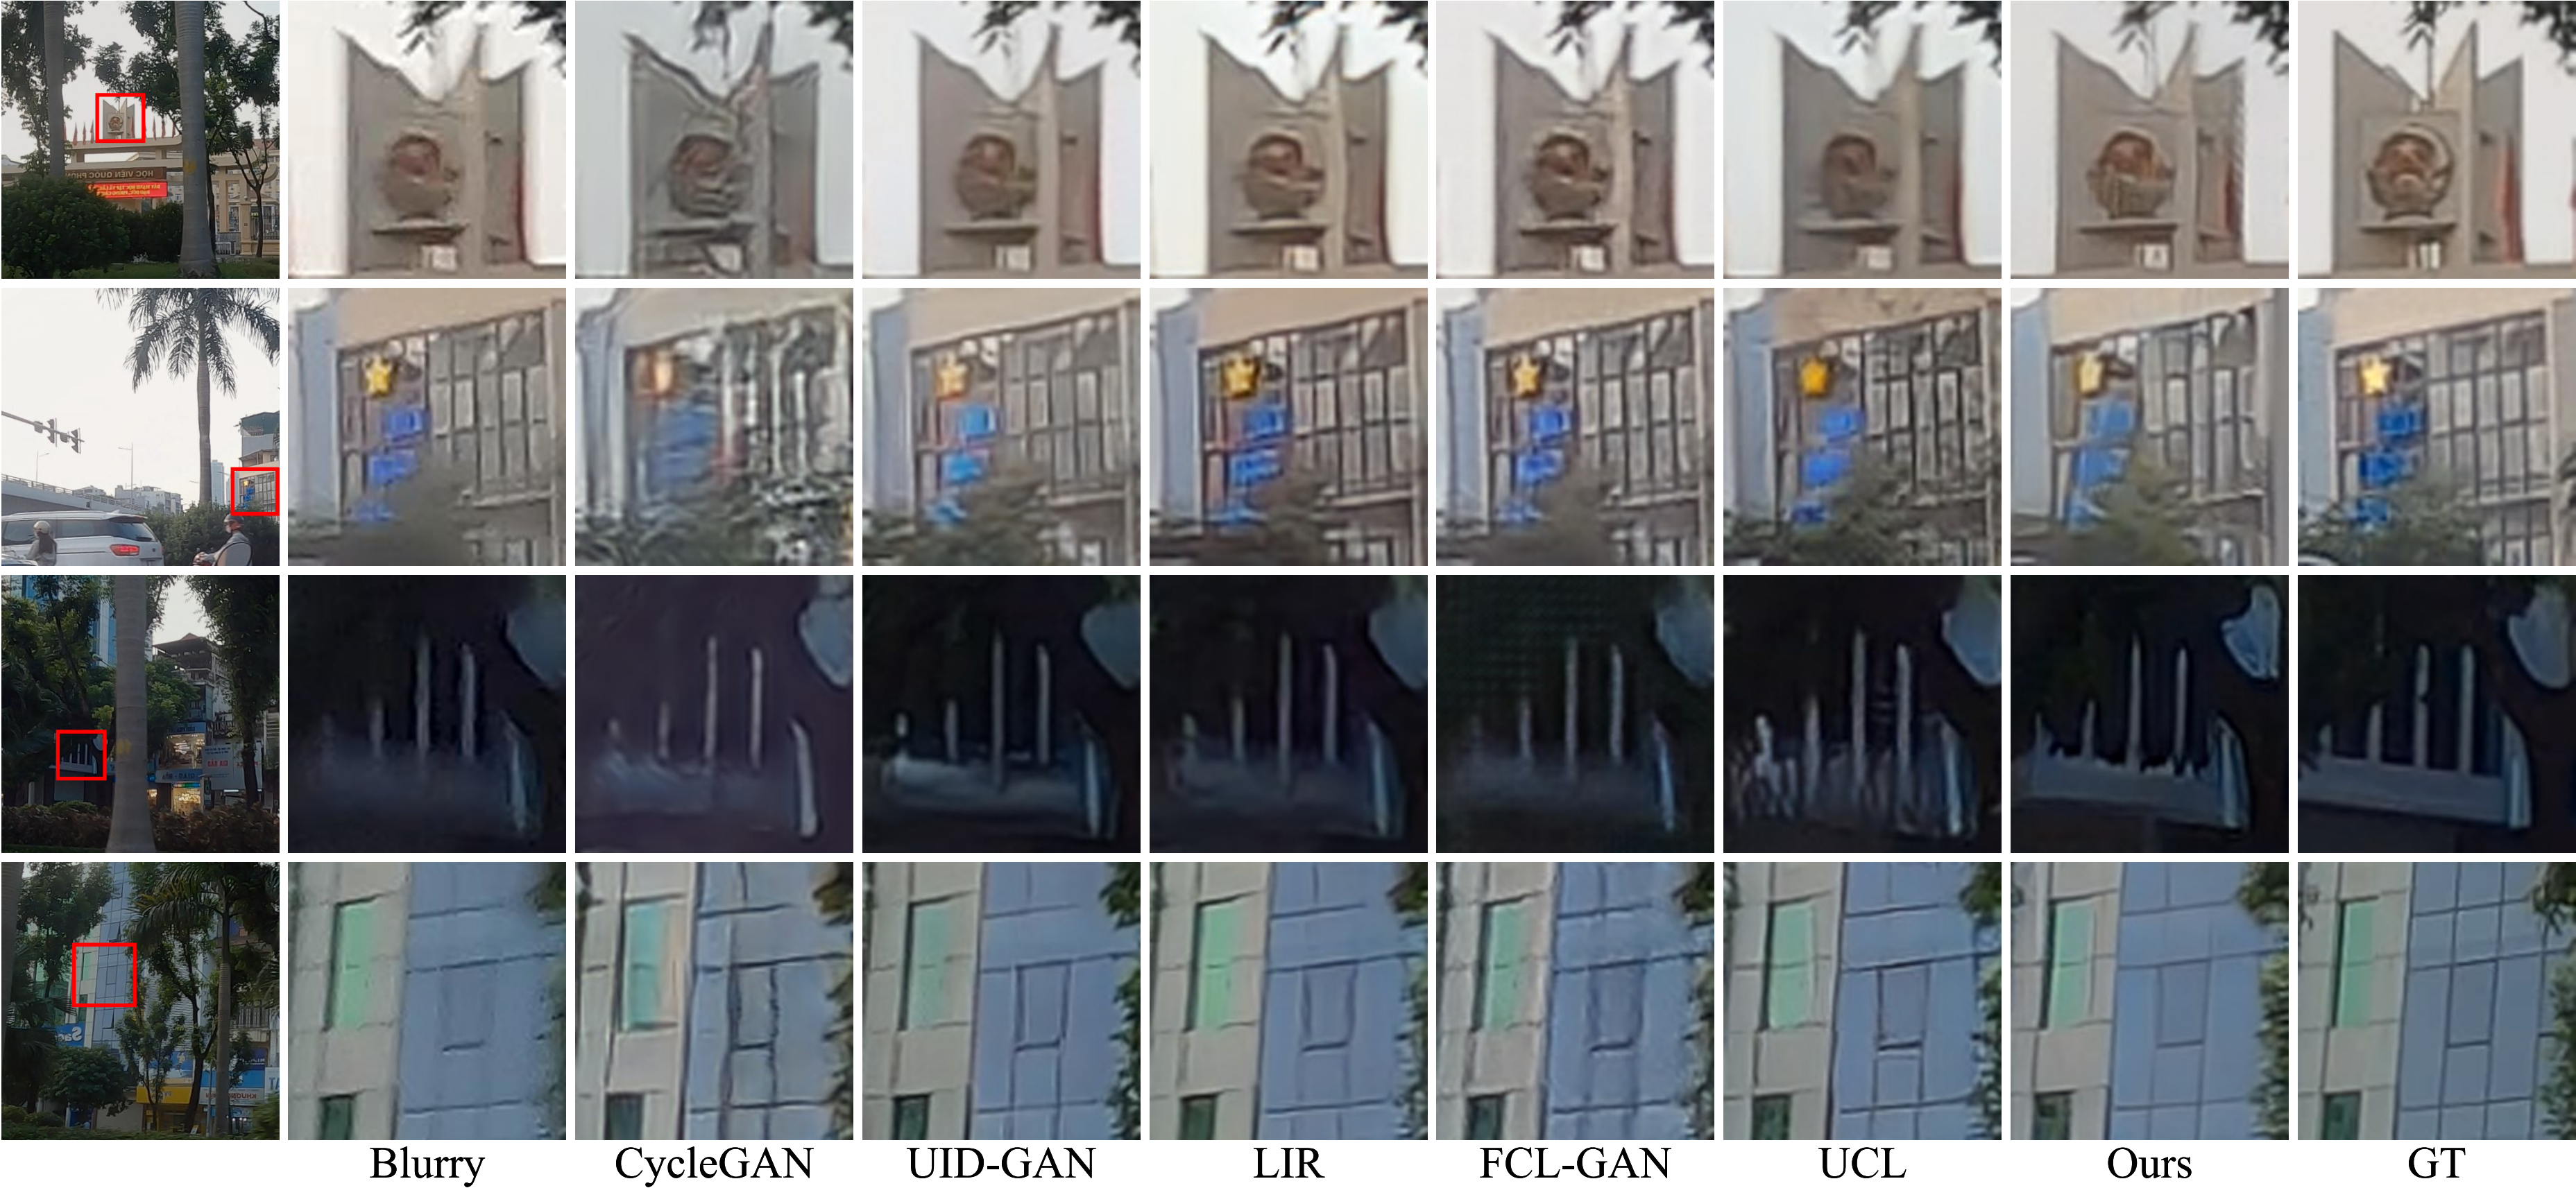

Blurry

CycleGAN

UID-GAN

LIR

FCL-GAN

UCL

Ours

GT

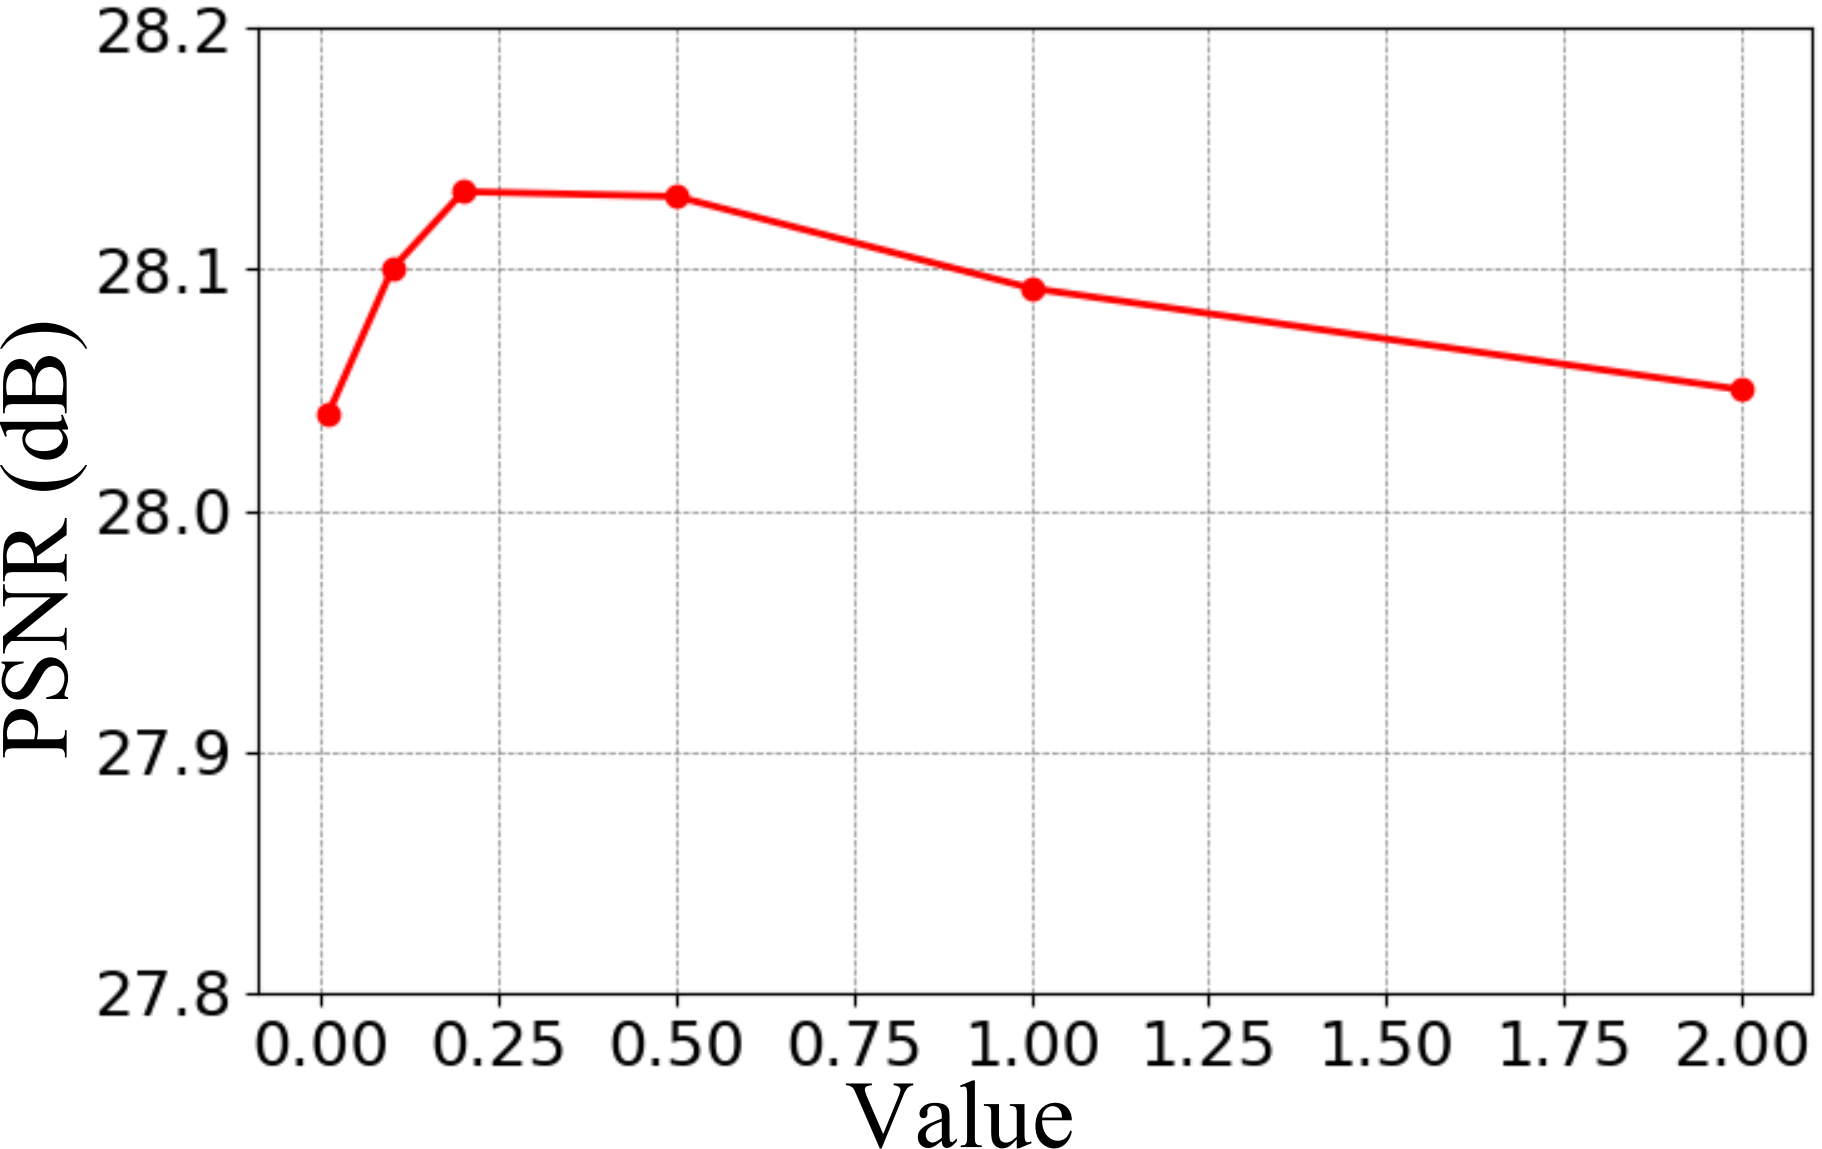

Supplement: Supplementary file 1 [file supp2.pdf]
